# Supplementary material for: Animal behavioral analysis and neural encoding with transformer-based self-supervised pretraining
Source: arXiv:2507.09513 source file (2026-02-27)

ResNet-50 (AP10K)

ViT-M (IN)

ViT-M (IN+PT)

BEAST

IBL 1000-Frame Finetune

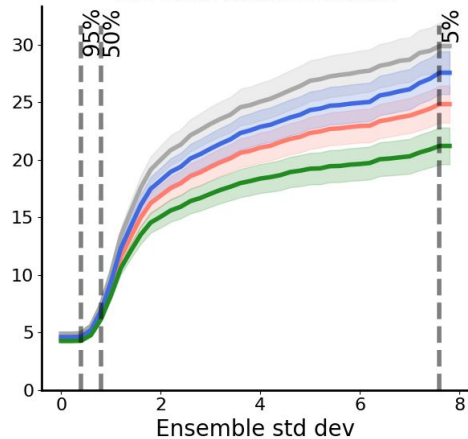

Mirror-mouse 789-Frame Finetune

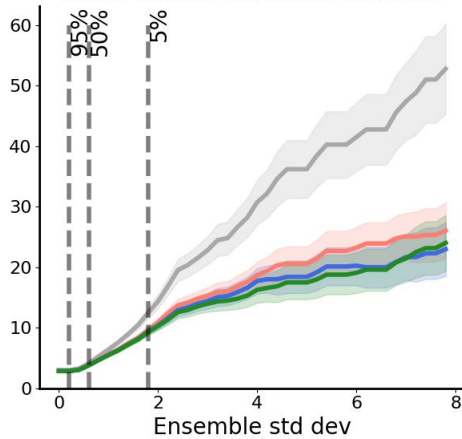

CRIM13 1000-Frame Finetune

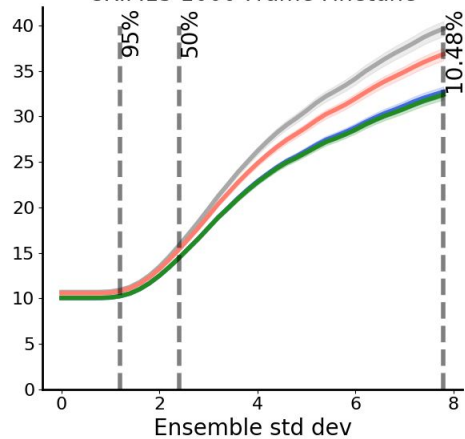

Mirror-fish 373-Frame Finetune

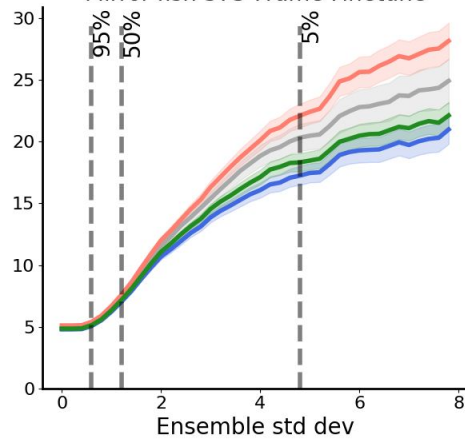

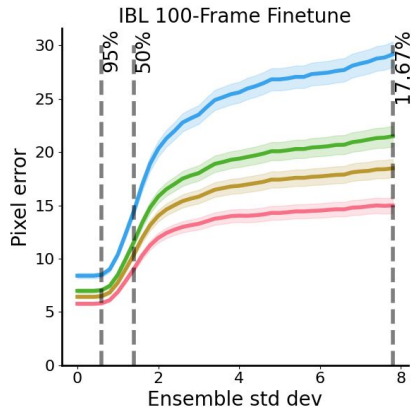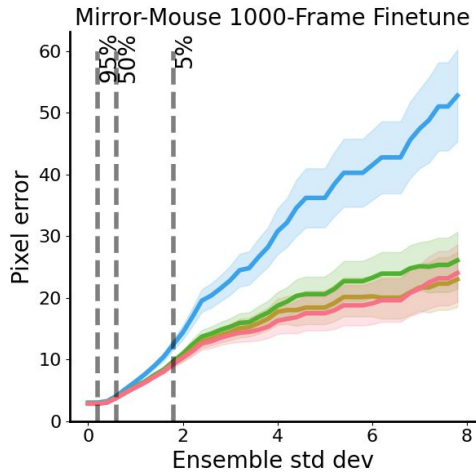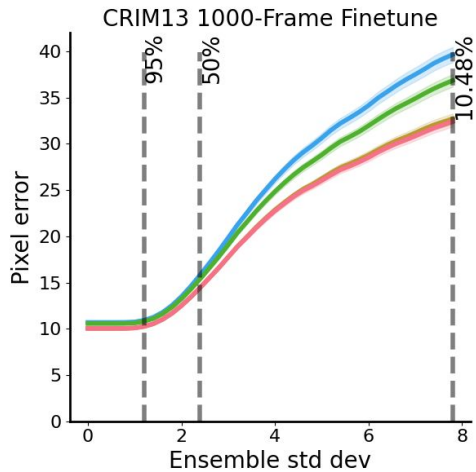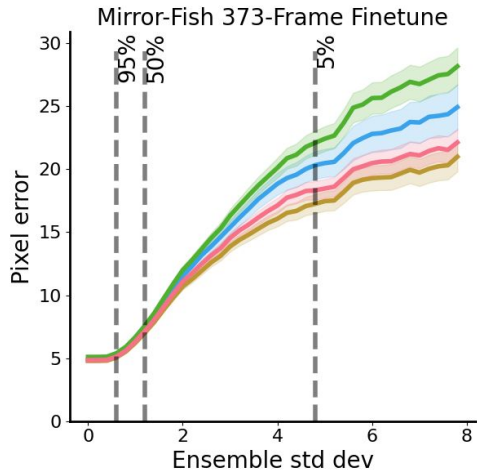

Supplement: Supplementary file 1 [file appendix_litpose.pdf]
